# Supplementary material for: TSFC: a structure-preserving form compiler
Source: arXiv:1705.03667 ancillary file (2018-04-09)
Supplement: Supplementary file 1 [file supplement.pdf]

# SUPPLEMENTARY MATERIALS: TSFC: A STRUCTURE-PRESERVING FORM COMPILER*

MIKLÓS HOMOLYA†, LAWRENCE MITCHELL‡, FABIO LUPORINI§, AND DAVID A. HAM¶

**SM1. Graph representation of UFL forms.** Figure SM1 and Figure SM2 show the graph representation of the Laplace operator as a UFL form before and after the application of pullbacks, corresponding to (1.6) and (1.7) respectively.

**SM2. Simple code generation.** Algorithm SM1 contains simple, but correct code generation for (4.2). This also has loop nests for `ListTensor` expressions, such as adjugate matrix $B$, $l_1$, and $l_2$. This is an intermediate step that is optimized further in subsection 4.3.

**SM3. C code generation.** Listing SM1 is a straightforward transcription of Algorithm 3 to C code. The definitions of compile-time constant tensors $C^{(1,1)}$, $C^{(1,2)}$, $C^{(2,1)}$, $C^{(2,2)}$, $w$, $E^{(1)}$, and $E^{(2)}$ are prepended to the function body. The element tensor $A$ and the local coordinate coefficients vector $c$ are defined as kernel arguments. Lines 10–14 may be omitted if the caller clears `A`.

**SM4. Test cases for experimental evaluation.** Here we provide the full description of the four test cases used for experimental evaluation.

**Helmholtz equation.**

$$a = (uv + \nabla u \cdot \nabla v)\,\mathrm{d}x \tag{SM4.1}$$

**Linear elasticity.** In elastic models the solution is typically a *displacement vector* field. Let $\mathbf{u}$ and $\mathbf{v}$ be vector-valued trial and test functions, and let $\varepsilon$ denote the symmetric part of the Jacobian of a vector field. Then the bilinear form is defined as follows:

$$\varepsilon(\mathbf{u}) = \frac{1}{2}\left[\nabla\mathbf{u} + (\nabla\mathbf{u})^T\right] \tag{SM4.2}$$

$$a = \varepsilon(\mathbf{u}) : \varepsilon(\mathbf{v})\,\mathrm{d}x \tag{SM4.3}$$

**Hyperelasticity.** A simple hyperelastic model. First, we define the strain energy

*Submitted to SIAM Journal on Scientific Computing on April 9, 2018.

**Funding:** This work was supported by The Grantham Institute; the Engineering and Physical Sciences Research Council [grant number EP/M011054/1]; the Department of Computing, Imperial College London; and the Natural Environment Research Council [grant number NE/K008951/1].

†The Grantham Institute and Department of Computing, Imperial College London, London, SW7 2AZ, UK (m.homolya14@imperial.ac.uk)

‡Department of Computing and Department of Mathematics, Imperial College London, London, SW7 2AZ, UK (lawrence.mitchell@imperial.ac.uk)

§Now at Department of Earth Science and Engineering, Imperial College London, London, SW7 2AZ, UK (f.luporini12@imperial.ac.uk)

¶Department of Mathematics, Imperial College London, London, SW7 2AZ, UK (david.ham@imperial.ac.uk)

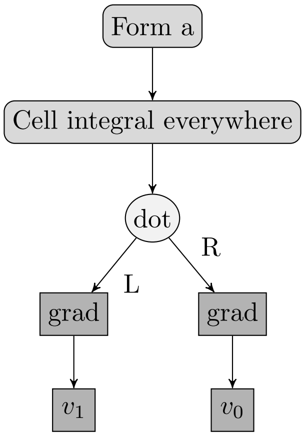


Figure SM1: *Tree representation* of the form (1.6).

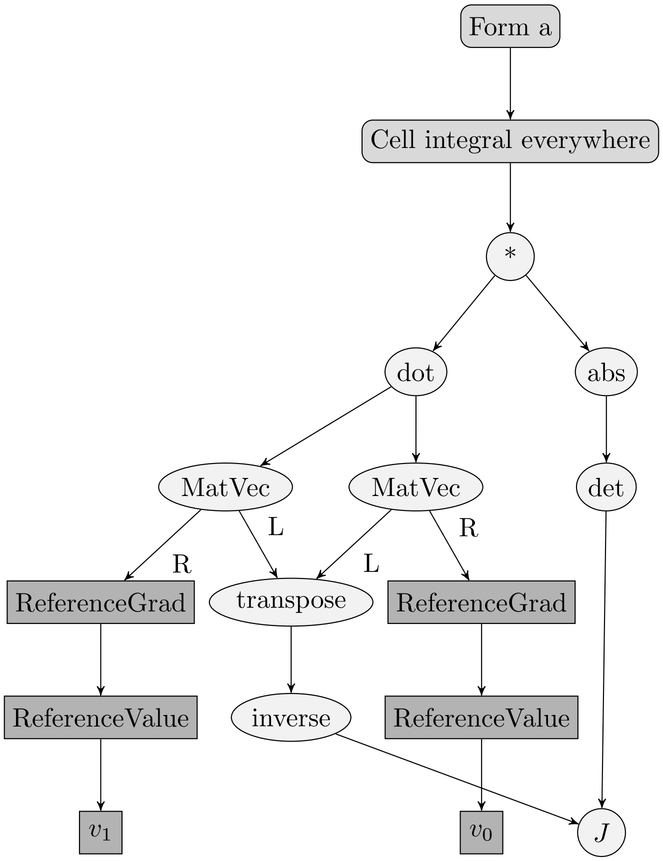


Figure SM2: The Laplace operator after changing to reference space, equivalent to (1.7). The presence of two references (arrows) to $J$ in place of replicating the $J$ node make this a *directed acyclic graph* (DAG) rather than a tree.

**Algorithm SM1** Simple code generation for the expression (4.2).

**for all** $q$ **do**
  $J^{(1,1)}[q] \leftarrow 0$
**for all** $q, r$ **do**
  $J^{(1,1)}[q] \mathrel{+}= C^{(1,1)}_{q,r} * c_r$
**for all** $q$ **do**
  $J^{(1,2)}[q] \leftarrow 0$
**for all** $q, r$ **do**
  $J^{(1,2)}[q] \mathrel{+}= C^{(1,2)}_{q,r} * c_r$
**for all** $q$ **do**
  $J^{(2,1)}[q] \leftarrow 0$
**for all** $q, r$ **do**
  $J^{(2,1)}[q] \mathrel{+}= C^{(2,1)}_{q,r} * c_r$
**for all** $q$ **do**
  $J^{(2,2)}[q] \leftarrow 0$
**for all** $q, r$ **do**
  $J^{(2,2)}[q] \mathrel{+}= C^{(2,2)}_{q,r} * c_r$
**for all** $q$ **do**
  $B[q, \ldots] \leftarrow \begin{bmatrix} J^{(2,2)}[q] & -J^{(1,2)}[q] \\ -J^{(2,1)}[q] & J^{(1,1)}[q] \end{bmatrix}$
**for all** $q, k$ **do**
  $l_1[q, k, \ldots] \leftarrow \begin{bmatrix} E^{(1)}_{q,k} & E^{(2)}_{q,k} \end{bmatrix}$
**for all** $i_5, q, k$ **do**
  $t_1[i_5, q, k] \leftarrow 0$
**for all** $i_3, i_5, q, k$ **do**
  $t_1[i_5, q, k] \mathrel{+}= B[q, i_3, i_5] \div (J^{(1,1)}[q] * J^{(2,2)}[q] - J^{(1,2)}[q] * J^{(2,1)}[q]) * l_1[q, k, i_3]$
**for all** $q, j$ **do**
  $l_2[q, j, \ldots] \leftarrow \begin{bmatrix} E^{(1)}_{q,j} & E^{(2)}_{q,j} \end{bmatrix}$
**for all** $i_5, q, j$ **do**
  $t_2[i_5, q, j] \leftarrow 0$
**for all** $i_4, i_5, q, j$ **do**
  $t_2[i_5, q, j] \mathrel{+}= B[q, i_4, i_5] \div (J^{(1,1)}[q] * J^{(2,2)}[q] - J^{(1,2)}[q] * J^{(2,1)}[q]) * l_2[q, j, i_4]$
**for all** $q, j, k$ **do**
  $t_3[q, j, k] \leftarrow 0$
**for all** $i_5, q, j, k$ **do**
  $t_3[q, j, k] \mathrel{+}= t_1[i_5, q, k] * t_2[i_5, q, j]$
**for all** $j, k$ **do**
  $A[j, k] \leftarrow 0$
**for all** $j, k, q$ **do**
  $A[j, k] \mathrel{+}= w_q * \mathrm{abs}(J^{(1,1)}[q] * J^{(2,2)}[q] - J^{(1,2)}[q] * J^{(2,1)}[q]) * t_3[q, j, k]$

---

function over the displacement vector field $\mathbf{u}$:

$$\mathbf{F} = \mathbf{I} + \nabla \mathbf{u} \quad \triangleright \text{Deformation gradient} \tag{SM4.4}$$

$$\mathbf{C} = \mathbf{F}^T \mathbf{F} \quad \triangleright \text{Right Cauchy-Green tensor} \tag{SM4.5}$$

$$\mathbf{E} = (\mathbf{C} - \mathbf{I})/2 \quad \triangleright \text{Euler-Lagrange strain tensor} \tag{SM4.6}$$

$$\Psi = \frac{\lambda}{2}[\mathrm{tr}(\mathbf{E})]^2 + \mu\, \mathrm{tr}(\mathbf{E}^2) \quad \triangleright \text{Strain energy function} \tag{SM4.7}$$

where $\lambda$ and $\mu$ are the *Lamé parameters*, and $\mathbf{I}$ is the identity matrix. Now, we define the Piola-Kirchhoff stress tensors:

$$\mathbf{S} = \frac{\partial \Psi}{\partial \mathbf{E}} \quad \triangleright \text{Second Piola-Kirchhoff stress tensor} \tag{SM4.8}$$

$$\mathbf{P} = \mathbf{F}\mathbf{S} \quad \triangleright \text{First Piola-Kirchhoff stress tensor} \tag{SM4.9}$$

One could, of course, derive that $\mathbf{S} = \lambda\, \mathrm{tr}(\mathbf{E})\mathbf{I} + 2\mu\mathbf{E}$, but we leave the symbolic differentiation for UFL. Finally, the residual form of this nonlinear problem is

$$r = \mathbf{P} : \nabla \mathbf{v} - \mathbf{b} \cdot \mathbf{v} \tag{SM4.10}$$

where $\mathbf{b}$ is the external forcing. To assemble a left-hand side, one must

**Listing SM1** Local assembly kernel for $\int \nabla u \cdot \nabla v \, \mathrm{d}x$ in C.

```
static inline void kernel(double A[4][4], const double c[8])
{
    static const double C11[4][8] = { ... };
    static const double C12[4][8] = { ... };
    static const double C21[4][8] = { ... };
    static const double C22[4][8] = { ... };
    static const double w[4] = { ... };
    static const double E1[4][4] = { ... };
    static const double E2[4][4] = { ... };
    for (int j = 0; j < 4; j++) {
        for (int k = 0; k < 4; k++) {
            A[j][k] = 0;
        }
    }
    for (int q = 0; q < 4; q++) {
        double J11 = 0;
        double J12 = 0;
        double J21 = 0;
        double J22 = 0;
        for (int r = 0; r < 8; r++) {
            J11 += C11[q][r]*c[r];
            J12 += C12[q][r]*c[r];
            J21 += C21[q][r]*c[r];
            J22 += C22[q][r]*c[r];
        }
        double B[2][2] = { { J22, -J12 }, { -J21, J11 } };
        double d = J11*J22 - J12*J21;
        double t1[4][2];
        for (int k = 0; k < 4; k++) {
            double l1[2] = { E1[q][k], E2[q][k] };
            for (int i_5 = 0; i_5 < 2; i_5++) {
                t1[k][i_5] = 0;
            }
            for (int i_3 = 0; i_3 < 2; i_3++) {
                for (int i_5 = 0; i_5 < 2; i_5++) {
                    t1[k][i_5] += (B[i_3][i_5]/d)*l1[i_3];
                }
            }
        }
        double t4 = w[q]*fabs(d);
        for (int j = 0; j < 4; j++) {
            double l2[2] = { E1[q][j], E2[q][j] };
            double t2[2];
            for (int i_5 = 0; i_5 < 2; i_5++) {
                t2[i_5] = 0;
            }
            for (int i_4 = 0; i_4 < 2; i_4++) {
                for (int i_5 = 0; i_5 < 2; i_5++) {
                    t2[i_5] += (B[i_4][i_5]/d)*l2[i_4];
                }
            }
            for (int k = 0; k < 4; k++) {
                double t3 = 0;
                for (int i_5 = 0; i_5 < 2; i_5++) {
                    t3 += t1[k][i_5]*t2[i_5];
                }
            A[j][k] += t4*t3;
        }
    }
}
```

linearize the residual around an *approximate* solution $\mathbf{u}$:

$$a = \delta r(\mathbf{u}; \delta\mathbf{u}) = \lim_{\epsilon \to 0} \frac{r(\mathbf{u} + \epsilon\delta\mathbf{u}) - r(\mathbf{u})}{\epsilon} \tag{SM4.11}$$

This bilinear form has trial function $\delta\mathbf{u}$, test function $\mathbf{v}$, and $\mathbf{u}$ is a coefficient of the form.

**Holzapfel-Ogden model.** A more complicated hyperelastic model described in [SM1]. Unlike the simple hyperelastic model, this model uses a volume-preserving right Cauchy–Green strain tensor:

$$J = \det(\mathbf{F}) \tag{SM4.12}$$
$$\bar{\mathbf{C}} = J^{-\frac{2}{3}} \mathbf{F}^T \mathbf{F} \tag{SM4.13}$$

Then defines the following rotation invariant functions:

$$I_1 = \mathrm{tr}(\bar{\mathbf{C}}) \tag{SM4.14}$$
$$I_{4f} = \mathbf{e}_f \cdot \bar{\mathbf{C}}\mathbf{e}_f \tag{SM4.15}$$
$$I_{4s} = \mathbf{e}_s \cdot \bar{\mathbf{C}}\mathbf{e}_s \tag{SM4.16}$$
$$I_{8fs} = \mathbf{e}_s \cdot \bar{\mathbf{C}}\mathbf{e}_f \tag{SM4.17}$$

where $\mathbf{e}_f$ and $\mathbf{e}_s$ denote unit vectors pointing in the local myocardial fiber and sheet directions, respectively. The strain energy function is defined as

$$\begin{aligned} \Psi =& \frac{a}{2b} \left(\exp\left[b(I_1 - 3)\right] - 1\right) \\ &+ \frac{h(I_{4f})a_f}{2b_f} \left(\exp\left[b_f(I_{4f} - 1)^2\right] - 1\right) \\ &+ \frac{h(I_{4s})a_s}{2b_s} \left(\exp\left[b_s(I_{4s} - 1)^2\right] - 1\right) \\ &+ \frac{a_{fs}}{2b_{fs}} \left(\exp\left[bI_{8fs}^2\right] - 1\right) \end{aligned} \tag{SM4.18}$$

where $h(x)$ is a Heaviside function with a jump at $x = 1$, and the material parameters are

$$m = (a, b, a_f, b_f, a_s, b_s, a_{fs}, b_{fs}).$$

We define the first Piola-Kirchhoff stress tensor, and the residual form without external forcing:

$$\mathbf{P} = \frac{\partial \Psi}{\partial \mathbf{F}} \qquad \triangleright \text{ Find first Piola-Kirchhoff tensor} \tag{SM4.19}$$
$$r = \mathbf{P} : \nabla \mathbf{v} \tag{SM4.20}$$

Finally, (SM4.11) gives the bilinear form again.

## REFERENCES

[SM1] G. Balaban, M. S. Alnæs, J. Sundnes, and M. E. Rognes, *Adjoint multi-start-based estimation of cardiac hyperelastic material parameters using shear data*, Biomechanics and Modeling in Mechanobiology, 15 (2016), pp. 1509–1521, https://doi.org/10.1007/s10237-016-0780-7, https://arxiv.org/abs/1603.03796.
